# Supplementary material for: Ergodic properties of linked-twist maps
Source: arXiv:0812.0899 source file (2008-12-04)
Supplement: Supplementary file 1 [file appendix1.tex]

\chapter{Appendix title}
\setcounter{equation}{0}
\setcounter{figure}{0}
\label{appendix1}

Appendix text
